# Supplementary material for: Bloch Oscillations of Driven Dissipative Solitons in a Synthetic Dimension
Source: arXiv:2112.10756 source file (2021-12-20)
Supplement: Supplementary file 1 [file SI.pdf]

# Supplementary Information – Bloch Oscillations of Driven Dissipative Solitons in a Synthetic Dimension

Nicolas Englebert,[1,*] Nathan Goldman,[2] Miro Erkintalo,[3,4] Nader Mostaan,[2,5,6] Simon-Pierre Gorza,[1] François Leo,[1] and Julien Fatome[3,4,7]

[1]*Service OPERA-Photonique, Université libre de Bruxelles (U.L.B.), 50 Avenue F. D. Roosevelt, CP 194/5, B-1050 Brussels, Belgium*
[2]*CENOLI, Université libre de Bruxelles (U.L.B.), CP 231, Campus Plaine, B-1050 Brussels, Belgium*
[3]*Department of Physics, University of Auckland, Auckland 1010, New Zealand*
[4]*The Dodd-Walls Centre for Photonic and Quantum Technologies, New Zealand*
[5]*Department of Physics and Arnold Sommerfeld Center for Theoretical Physics (ASC), Ludwig-Maximilians-Universität München, Theresienstr. 37, D-80333 München, Germany*
[6]*Munich Center for Quantum Science and Technology (MCQST), Schellingstr. 4, D-80799 München, Germany*
[7]*Laboratoire Interdisciplinaire Carnot de Bourgogne, UMR 6303 CNRS – Université Bourgogne-Franche-Comté, Dijon, France*

This document contains Supplementary Information for the manuscript entitled "Bloch Oscillations of Driven Dissipative Solitons in a Synthetic Dimension". We derive the cavity soliton equations of motion based on a Lagrangian-approach and provide a detailed version of the experimental set-up depicted in Fig. 1 of the main manuscript. We also present additional experimental result that demonstrate CSs in the presence of a synthetic frequency dimension that involves all the cavity modes, realised by configuring the intra-cavity modulator to couple nearest-neighbour modes.

## A. Cavity soliton Bloch oscillations based on a Lagrangian approach

We first present a brief derivation of the equations of motion that describe the evolution of CSs in the synthetic (frequency) space and the dual (fast-time) space, i.e., Eqs. (4) of the main manuscript. Our starting point is the generalised Lugiato-Lefever equation (LLE, Eq. (6) of the main manuscript) [1, 2] with a fast-time modulated detuning term to account for the intra-cavity phase modulation [3]:

$$it_{\mathrm{R}}\frac{\partial A}{\partial t} - \frac{\beta_2 L_c}{2}\frac{\partial^2 A}{\partial \tau^2} + \gamma L_c|A|^2 A = -i\frac{\Lambda_e}{2}A + iS + [\delta_0 - J_{\mathrm{EOM}}\cos(\Omega_m(\tau - Ft))]A. \tag{S1}$$

Here $A(t,\tau)$ describes the electric field envelope of the intra-cavity field in the dual (fast-time) space, $L_c$ is the resonator circumference, and $t_{\mathrm{R}} = \mathrm{FSR}^{-1}$ is the roundtrip time at the driving wavelength. $\beta_2$ and $\gamma$ are respectively the group-velocity dispersion and the nonlinear Kerr coefficient of the resonator waveguide, $\Lambda_{\mathrm{e}}$ denotes the effective cavity loss [4] expressed as a proportion of light intensity dissipated each roundtrip, $S = \sqrt{\theta P_{\mathrm{in}}}$ where $\theta$ and $P_{\mathrm{in}}$ correspond respectively to the input coupler ratio and the power of the coherent driving field, and $\delta_0$ is the mean-value of the phase detuning between the driving field and a cavity resonance. The last term in Eq. (S1) describes the effect of the electro-optic modulator (EOM) that phase modulates the intra-cavity field with amplitude $J_{\mathrm{EOM}}$ and frequency $f_{\mathrm{EOM}} = m \times \mathrm{FSR} + \Delta f$, with $m \in \mathbb{N}$ and $\Delta f$ a frequency offset between $f_{\mathrm{EOM}}$ and the $m^{\mathrm{th}}$ harmonic of the cavity FSR. The modulation frequency $f_{\mathrm{EOM}}$ defines the effective inter-site distance of the synthetic lattice viz. $\Omega_m = 2\pi \times m \times \mathrm{FSR}$ and the effective force viz. $F = \Delta f / f_{\mathrm{EOM}} \approx \Delta f/(m\mathrm{FSR})$. Note that Eq. (S1) is expressed in a reference frame moving at the group velocity of light at the driving frequency.

There are no closed-form analytical expressions known that would describe the cavity soliton (CS) solutions of Eq. (S1). However, an approximate solution can be found using a perturbative Lagrangian approach [5]. We derive the CS equations of motion pertinent to our work by generalising this method to include the modulation of the detuning. To this end, we define the following perturbation that differentiates Eq. (S1) from the integrable nonlinear Schrödinger equation (whose soliton solutions are well known):

$$\mathcal{R} = -i\frac{\Lambda_e}{2}A + iS - J_{\mathrm{EOM}}\cos(\Omega_m(\tau - Ft))A. \tag{S2}$$

---

*Electronic address: nicolas.englebert@ulb.be

The Lagrangian density of the system is given by [5, 6]

$$\mathcal{L}(A) = \frac{it_{\mathrm{R}}}{2}\left(A^*\frac{\partial A}{\partial t} - A\frac{\partial A^*}{\partial t}\right) + \frac{\beta_2 L_c}{2}\left|\frac{\partial A}{\partial \tau}\right|^2 + \frac{\gamma L_c}{2}|A|^4 - \delta_0|A|^2, \tag{S3}$$

such that $\delta\mathcal{L}/\delta A^* = \mathcal{R}$ is equivalent to Eq. (S1) [7].

To derive the CS equations of motion, we use the ansatz [5, 6]:

$$A_s(t,\tau) = B\,\mathrm{sech}\left(\frac{\tau - \langle\tau\rangle}{\tau_s}\right)\mathrm{e}^{-i\langle\omega\rangle(\tau-\langle\tau\rangle)}\mathrm{e}^{i\phi} \tag{S4}$$

where $\langle\omega\rangle$ corresponds to the soliton central frequency (centre of mass), $B$ is the soliton amplitude (with units of $\mathrm{W}^{1/2}$), $\langle\tau\rangle$ is the soliton position along the dual (fast-time) domain, $\tau_s$ is the soliton's temporal duration and $\phi$ is an additional phase. All these parameters depend on the slow-time variable $t$. Note that $A_s$ is an exact solution of Eq. (S1) in the absence of the perturbation ($\mathcal{R} = 0$), provided that the amplitude $B$ and duration $\tau_s$ satisfy the well-known soliton condition of the nonlinear Schrödinger equation. It is also worth noting that CSs sit atop a continuous-wave (CW) background whose amplitude decreases when the detuning is increased [8, 9]; accordingly, the ansatz given by Eq. (S4) is particularly accurate in the large detuning limit where the CW background can be neglected.

The equations of motion for each of the CS parameters $\{r_i\} = \{B(t), \langle\omega\rangle(t), \langle\tau\rangle(t), \phi(t)\}$ can be obtained from [5, 6]

$$\frac{\partial L}{\partial r_i} - \frac{d}{dt}\frac{\partial L}{\partial \dot{r_i}} = \int\left(\mathcal{R}\frac{\partial A_s^*}{\partial r_i} + \mathcal{R}^*\frac{\partial A_s}{\partial r_i}\right)\mathrm{d}t \tag{S5}$$

where $L = \int \mathcal{L}(A_s)\,\mathrm{d}t$ is Lagrangian. Together with Eq. (S3) and Eq. (S4), we find

$$L = 2B^2\tau_s\left(\frac{2\gamma L_c B^2}{2} + \frac{\beta_2 L_c}{2}\left(\frac{1}{3\tau_s^2} + \langle\omega\rangle^2\right) - t_R\langle\omega\rangle\frac{\partial\langle\tau\rangle}{\partial t} - t_R\frac{\partial\phi}{\partial t}\right) \tag{S6}$$

Equation (S6) can be further simplified as the CS' amplitude and its temporal duration are related through the soliton condition $B\tau_s = \eta = \sqrt{(-\beta_2)/\gamma}$, leading to [6]

$$L = 2B\sqrt{\frac{-\beta_2}{\gamma}}\left(\frac{\gamma L_c B^2}{6} + \frac{\beta_2 L_c}{2}\langle\omega\rangle^2 - \delta_0 - t_R\langle\omega\rangle\frac{\partial\langle\tau\rangle}{\partial t} - t_R\frac{\partial\phi}{\partial t}\right) \tag{S7}$$

In what follows, we only detail the calculations pertinent to the parameter $\langle\tau\rangle$ as this calculation leads to the equation of motion of the frequency shift $\langle\omega\rangle$ experienced by the CS in the presence of an effective force ($F \neq 0$). The equations of motions obtained for the other parameters ($B(t), \langle\tau\rangle(t), \phi(t)$) are identical to those given in [6]. Considering our ansatz Eq. (S4), the perturbation Eq. (S2) now reads

$$\begin{aligned}\mathcal{R} &= -\frac{i\Lambda_e B}{2}\,\mathrm{sech}^2\left(\frac{\tau-\langle\tau\rangle}{\tau_s}\right) + i\,\mathrm{sech}\left(\frac{\tau-\langle\tau\rangle}{\tau_s}\right)\mathrm{e}^{-i\langle\omega\rangle(\tau-\langle\tau\rangle)}\mathrm{e}^{i\phi} - J_{\mathrm{EOM}}B\,\mathrm{sech}^2\left(\frac{\tau-\langle\tau\rangle}{\tau_s}\right)\cos(\Omega_m(t-Ft))\\ \mathcal{R}^* &= \frac{i\Lambda_e B}{2}\,\mathrm{sech}^2\left(\frac{\tau-\langle\tau\rangle}{\tau_s}\right) - i\,\mathrm{sech}\left(\frac{\tau-\langle\tau\rangle}{\tau_s}\right)\mathrm{e}^{i\langle\omega\rangle(\tau-\langle\tau\rangle)}\mathrm{e}^{-i\phi} - J_{\mathrm{EOM}}B\,\mathrm{sech}^2\left(\frac{\tau-\langle\tau\rangle}{\tau_s}\right)\cos(\Omega_m(t-Ft))\end{aligned} \tag{S8}$$

The derivative of $A_s$ and its complex conjugate with respect to $\langle\tau\rangle$ appearing in the right-hand side of Eq. (S5) are

$$\begin{aligned}\frac{\partial A_s}{\partial\langle\tau\rangle} &= \frac{B}{\tau_s}\,\mathrm{sech}\left(\frac{\tau-\langle\tau\rangle}{\tau_s}\right)\tanh\left(\frac{\tau-\langle\tau\rangle}{\tau_s}\right)\mathrm{e}^{-i\langle\omega\rangle(\tau-\langle\tau\rangle)}\mathrm{e}^{i\phi} + i\langle\omega\rangle B\,\mathrm{sech}\left(\frac{\tau-\langle\tau\rangle}{\tau_s}\right)\mathrm{e}^{-i\langle\omega\rangle(\tau-\langle\tau\rangle)}\mathrm{e}^{i\phi}\\ \frac{\partial A_s^*}{\partial\langle\tau\rangle} &= \frac{B}{\tau_s}\,\mathrm{sech}\left(\frac{\tau-\langle\tau\rangle}{\tau_s}\right)\tanh\left(\frac{\tau-\langle\tau\rangle}{\tau_s}\right)\mathrm{e}^{i\langle\omega\rangle(\tau-\langle\tau\rangle)}\mathrm{e}^{-i\phi} - i\langle\omega\rangle B\,\mathrm{sech}\left(\frac{\tau-\langle\tau\rangle}{\tau_s}\right)\mathrm{e}^{i\langle\omega\rangle(\tau-\langle\tau\rangle)}\mathrm{e}^{-i\phi}\end{aligned} \tag{S9}$$

Therefore

$$\begin{aligned}\int\left(\mathcal{R}\frac{\partial A_s^*}{\partial\langle\tau\rangle} + \mathcal{R}^*\frac{\partial A_s}{\partial\langle\tau\rangle}\right)\mathrm{d}t = &-\frac{\Lambda_e\langle\omega\rangle B^2}{2}\int\mathrm{sech}^2\left(\frac{\tau-\langle\tau\rangle}{\tau_s}\right)\mathrm{d}t\\ &-\frac{2J_{\mathrm{EOM}}B^2}{\tau_s}\int\mathrm{sech}^2\left(\frac{\tau-\langle\tau\rangle}{\tau_s}\right)\tanh\left(\frac{\tau-\langle\tau\rangle}{\tau_s}\right)\cos(\Omega_m(t-Ft))\,\mathrm{d}t\\ &-\frac{2SB}{\tau_s}\int\mathrm{sech}\left(\frac{\tau-\langle\tau\rangle}{\tau_s}\right)\tanh\left(\frac{\tau-\langle\tau\rangle}{\tau_s}\right)\sin(\langle\omega\rangle(\tau-\langle\tau\rangle)-\phi)\,\mathrm{d}t\\ &-2S\langle\omega\rangle B\int\mathrm{sech}\left(\frac{\tau-\langle\tau\rangle}{\tau_s}\right)\cos(\langle\omega\rangle(\tau-\langle\tau\rangle)-\phi)\,\mathrm{d}t\end{aligned} \tag{S10}$$

After integration of Eq. (S9), we obtain

$$\int \left(\mathcal{R}\frac{\partial A_s^*}{\partial\langle\tau\rangle}+\mathcal{R}^*\frac{\partial A_s}{\partial\langle\tau\rangle}\right)\mathrm{d}t=-2\Lambda_e\langle\omega\rangle B^2\tau_s+J_{\mathrm{EOM}}B^2\Omega_m^2\tau_s^2\pi\mathrm{csch}\left(\frac{\Omega_m\tau_s\pi}{2}\right)\sin(\Omega_m(\langle\tau\rangle-Ft)) \tag{S11}$$

It remains to calculate the left-hand side of Eq. (S5)

$$\frac{\partial L}{\partial\langle\tau\rangle}-\frac{d}{dt}\frac{\partial L}{\partial\left(\frac{\partial\langle\tau\rangle}{\partial t}\right)}=2\langle\omega\rangle\sqrt{\frac{-\beta_2}{\gamma}}t_R\frac{dB}{dt}+2B\sqrt{\frac{-\beta_2}{\gamma}}t_R\frac{d\langle\omega\rangle}{dt} \tag{S12}$$

By eliminating $\tau_s$ from these equations, we find the equation of motion of the frequency shift $\langle\omega\rangle$ due to the phase modulation

$$t_R\frac{d(\langle\omega\rangle B)}{dt}=-\Lambda_e B\langle\omega\rangle+\pi\sqrt{\frac{-\beta_2}{\gamma}}\frac{J_{\mathrm{EOM}}\Omega_m^2}{2}\mathrm{csch}\left(\frac{\Omega_m\tau_s\pi}{2}\right)\sin(\Omega_m(\langle\tau\rangle-Ft)). \tag{S13}$$

Performing the same procedure for the three other parameters, we find the following four equations of motion, out of which only first one is impacted by the phase modulation

$$\begin{aligned}
t_R\frac{d\langle\omega\rangle}{dt}&=-\frac{\langle\omega\rangle}{B}t_R\frac{dB}{dt}+\frac{1}{B}\left(-\Lambda_e B\langle\omega\rangle+\pi\sqrt{\frac{-\beta_2}{\gamma}}\frac{J_{\mathrm{EOM}}\Omega_m^2}{2}\mathrm{csch}\left(\sqrt{\frac{-\beta_2}{\gamma}}\frac{\pi\Omega_m}{2B}\right)\sin(\Omega_m(\langle\tau\rangle-Ft))\right),\\
t_R\frac{dB}{dt}&=-\Lambda_e B+\pi S\cos(\phi)\,\mathrm{sech}\left(\sqrt{\frac{-\beta_2}{\gamma}}\frac{\langle\omega\rangle\pi}{2B}\right),\\
t_R\frac{d\phi}{dt}&=\frac{\gamma L_c B^2}{2}+\frac{\beta_2 L_c}{2}\langle\omega\rangle-\delta_0-t_R\langle\omega\rangle\frac{\partial\langle\tau\rangle}{\partial t},\\
t_R\frac{d\langle\tau\rangle}{dt}&=\beta_2 L_c\langle\omega\rangle.
\end{aligned} \tag{S14}$$

Since (i) the intra-cavity phase modulation can be interpreted as a detuning change along the fast-time domain $\tau$ and (ii) the CS's amplitude depends on the detuning, we might expect the amplitude parameter $B$ to be affected accordingly. However, in practice, the modulation amplitude $J_{\mathrm{EOM}}$ remains small with respect to the cavity detuning $\delta_0$, such that the CS's amplitude can be considered to be constant i.e. $dB/dt\approx 0$. Furthermore, since the assumption of large detuning is equivalent to assuming $\phi$ close to zero [6], the above system can be reduced to only two equations of motion:

$$\begin{aligned}
t_R\frac{d\langle\omega\rangle}{dt}&=-\Lambda_e\langle\omega\rangle+\pi\eta\frac{J_{\mathrm{EOM}}\Omega_m^2}{2B}\mathrm{csch}\left(\eta\frac{\pi\Omega_m}{2B}\right)\sin(\Omega_m(\langle\tau\rangle-Ft)),\\
t_R\frac{d\langle\tau\rangle}{dt}&=\beta_2 L_c\langle\omega\rangle.
\end{aligned} \tag{S15}$$

So far, all the equations have been written in a reference frame that moves with the group velocity of light at the driving frequency. In this reference frame, the intra-cavity phase modulation imparted by the EOM drifts in the fast-time domain in the presence of a desynchronisation ($F\neq 0$), as is evident in the equations written above. To gain more insights, it is convenient to introduce the following change of variable so as to shift into a reference frame where the phase modulation is stationary

$$\langle\tau\rangle\to\langle\tau\rangle-Ft \tag{S16}$$

With this change of variable, Eq. (S1) becomes the Eq. (7) of the main manuscript, while Eqs. (S15) become

$$t_{\mathrm{R}}\frac{d\langle\omega\rangle}{dt}=-\Lambda_{\mathrm{e}}\langle\omega\rangle+\Gamma\sin(\Omega_m\langle\tau\rangle),\qquad t_{\mathrm{R}}\frac{d\langle\tau\rangle}{dt}=t_{\mathrm{R}}F+\beta_2 L_c\langle\omega\rangle, \tag{S17}$$

where we introduced the coefficient

$$\Gamma=\pi\eta J_{\mathrm{EOM}}\frac{\Omega_m^2}{2B}\,\mathrm{csch}\left(\pi\eta\frac{\Omega_m}{2B}\right). \tag{S18}$$

The soliton duration is much smaller than the modulation period. Therefore, $\pi\eta\Omega_m/(2B)$ is small, thus yielding after a first-order Taylor-series expansion $\Gamma \approx J_{\mathrm{EOM}}\Omega_m$. With this approximation, Eqs. (S17) become identical to the transport Eqs. (4) of the main manuscript.

As noted in the main manuscript, in the limit of a small effective force ($F \sim 0$), the frequency variable $\langle\omega\rangle$ evolves slowly, allowing to approximate $d\langle\omega\rangle/dt \approx 0$. This yields the Adler-like synchronisation equation [10–12] for the temporal variable $\langle\tau\rangle$ [Eq. (5) of the main manuscript]

$$t_{\mathrm{R}}\frac{d\langle\tau\rangle}{dt} = Ft_{\mathrm{R}} + \beta_2 L_c \frac{J_{\mathrm{EOM}}\Omega_m}{\Lambda_{\mathrm{e}}}\sin(\Omega_m\langle\tau\rangle). \tag{S19}$$

Equation (S19) shows that the solitons' drift velocity in the fast-time domain is proportional to the derivative of detuning modulation. This result – derived using the Lagrangian approach – is commensurate with results obtained from a complementary CS perturbation theory that predicts the solitons to drift along parameter gradients with a velocity proportional to the gradient at the soliton position [12].

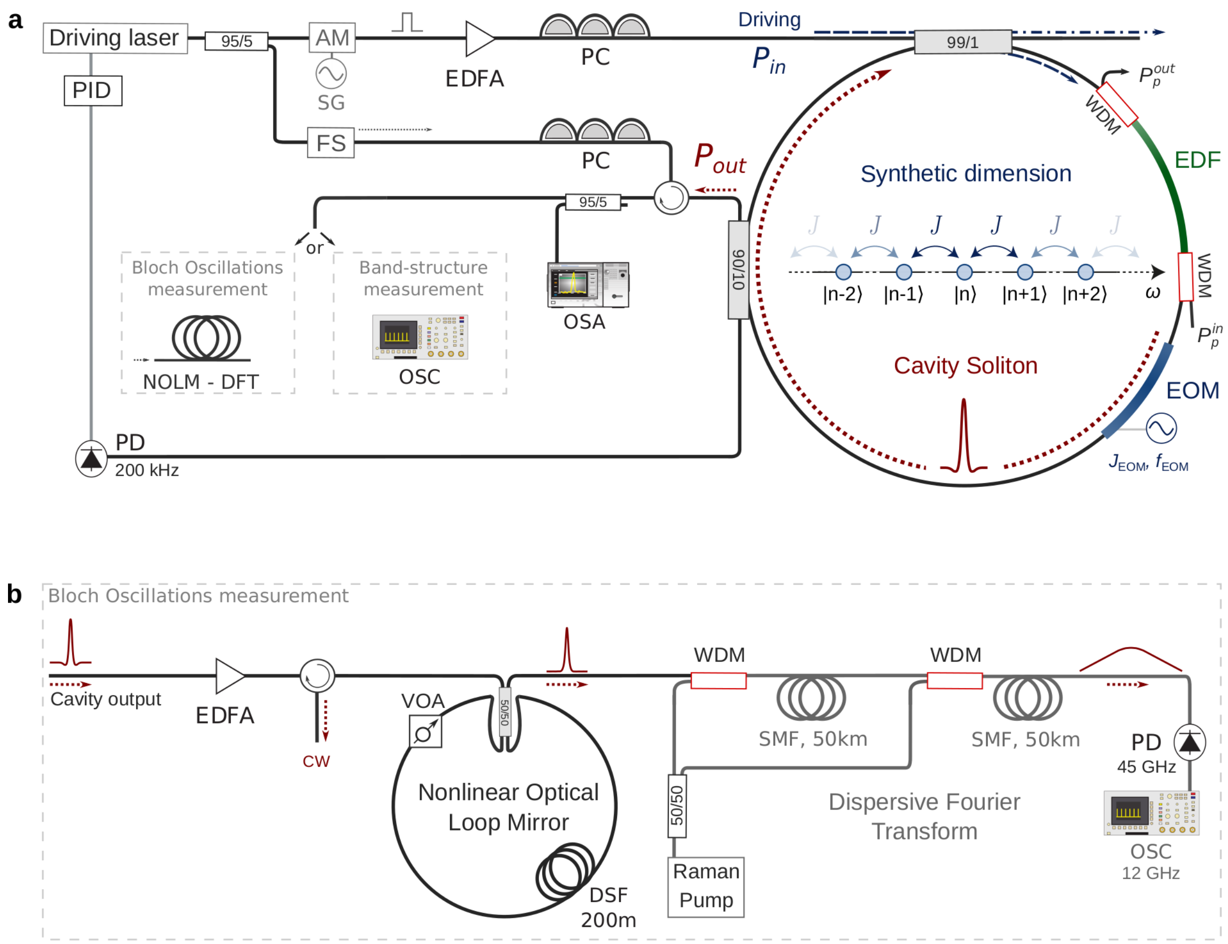


**Fig. S1. Complete experimental set-up.** **a**, Our synthetic frequency dimension is implemented within a 64-m-long [$\sim$ 63 m of standard telecommunication single-mode fibre (SMF-28) and a 75 cm-long segment of erbium doped fibre (EDF), pumped by a 1480 nm laser] active fibre ring cavity [4]. It is coherently-driven by means of a low-linewidth continuous wave (CW) laser centred at 1550.12 nm. This CW laser is modulated using an amplitude modulator (AM) driven by a signal generator (SG) whose frequency is an exact integer harmonic of the cavity free-spectral range (FSR). The pulsed driving beam is then amplified by means of a commercial erbium doped fibre amplifier (EDFA). Before being injected into the cavity through the 99/1 input coupler, the polarisation state is adjusted using a polarisation controller (PC). The resonator includes an electro-optic phase modulator (EOM) driven by a second signal generator, whose amplitude ($J_{\mathrm{EOM}}$) and frequency ($f_{\mathrm{EOM}}$) can be freely chosen. A detuning stabilisation is achieved by the means of a counter-propagative control signal, generated by frequency-shifting (FS) a small part of the driving laser power (5%) [13]. The polarisation state of the control signal is set to be identical to the one of the driving signal. Part of the intra-cavity power ($P_{\mathrm{out}}$) is extracted at the output coupler (90/10) to perform temporal and spectral diagnostics but also to actively stabilise the cavity detuning using a proportional-integral-derivative (PID) controller, driven by a 200 kHz photodiode. The optical spectrum is measured with an optical spectrum analyser (OSA). To measure the band structure (see Fig. 2a), the output power is sent to a 45 GHz photodiode connected to a 12 GHz real-time oscilloscope (OSC). **b**, To measure the cavity soliton Bloch oscillations (see Figs. 3a-d of the main manusript), the cavity output power is first amplified by a commercial EDFA. Then, the CW component (i.e. the driving field) is removed using a nonlinear optical loop mirror (NOLM, see Methods of the main manuscript). The background-free cavity soliton then propagates through $2 \times 50$ km segments of single-mode fibre (SMF) in order to realise dispersive Fourier transformation (DFT). To facilitate the DFT masurements, the CS signal is amplified in the SMF segments by means of Raman amplification, realised by adding a powerful 1455 nm CW laser through a wavelength division multiplexing (WDM) to co-propagate with the CSs. The 1455 nm Raman pump is the same for both SMF segments and its power is divided in two by a 50/50 coupler. After the propagation, the temporal signal is finally recorded by a 45 GHz photodiode connected to a 12 GHz real-time oscilloscope (OSC).

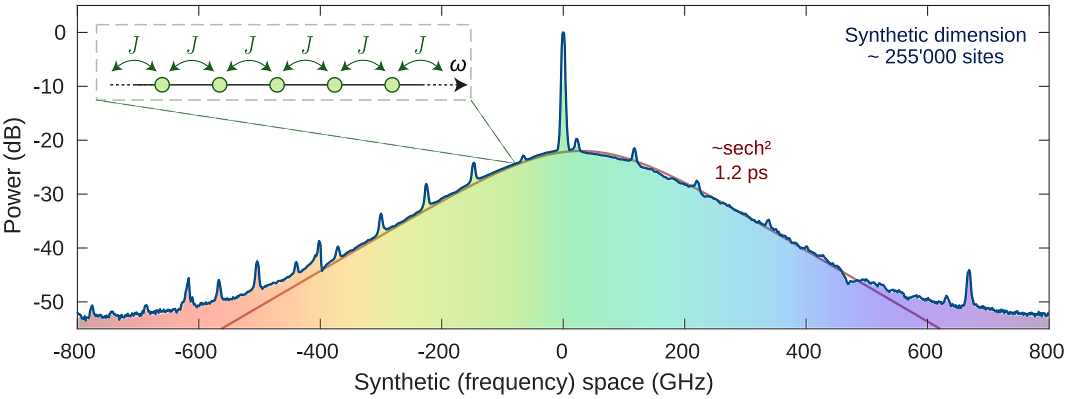


**Fig. S2. Cavity solitons in a synthetic dimension with nearest-neighbour cavity mode coupling.** Measured cavity soliton optical spectrum with $f_{\mathrm{EOM}} = 1 \times \mathrm{FSR}$. The soliton spectrum encompasses more than 250,000 equally-space synthetic lattice sites above the -15 dB level. A sech-squared fit (red) reveals the presence of a 1.2 ps-long pulse propagating indefinitely in the resonator. In contrast to the other experiments, where the cavity is driven with flat top pulses, the resonator is here driven by a continuous wave laser through the input coupler (here, the 90/10 coupler). The resonator differs from the one shown in Figure 1a in two points: (i) an isolator prevents the build-up of Brillouin scattering and (ii) a 1530/1550 nm wavelength division multiplexer (WDM) is added to send addressing pulses for deterministic soliton excitation. As the isolator prevents the use of a counter-propagating control signal, the resonator's response is used as a feedback signal for the PID controller. Once stabilised, a single cavity soliton can be addressed by picking a single pulse from a commercial picosecond laser using an acousto-optic modulator. It is then amplified before being sent into the cavity through the WDM [8]. Experimental parameters: $F = 0$, $f_{\mathrm{EOM}} = 3.1\,\mathrm{MHz}$, $J_{\mathrm{EOM}} = 0.6$ rad and $\theta P_{\mathrm{in}} = 10$ mW.

---


[1] Lugiato, L. A. & Lefever, R. Spatial Dissipative Structures in Passive Optical Systems. *Physical Review Letters* **58**, 2209–2211 (1987). URL `https://link.aps.org/doi/10.1103/PhysRevLett.58.2209`. Publisher: American Physical Society.

[2] Haelterman, M., Trillo, S. & Wabnitz, S. Dissipative modulation instability in a nonlinear dispersive ring cavity. *Optics Communications* **91**, 401–407 (1992). URL `http://www.sciencedirect.com/science/article/pii/003040189290367Z`.

[3] Tusnin, A. K., Tikan, A. M. & Kippenberg, T. J. Nonlinear states and dynamics in a synthetic frequency dimension. *Physical Review A* **102**, 023518 (2020). URL `https://link.aps.org/doi/10.1103/PhysRevA.102.023518`. Publisher: American Physical Society.

[4] Englebert, N., Mas Arabí, C., Parra-Rivas, P., Gorza, S.-P. & Leo, F. Temporal solitons in a coherently driven active resonator. *Nature Photonics* 1–6 (2021). URL `https://www.nature.com/articles/s41566-021-00807-w`. Publisher: Nature Publishing Group.

[5] Matsko, A. B. & Maleki, L. On timing jitter of mode locked Kerr frequency combs. *Optics Express* **21**, 28862–28876 (2013). URL `https://www.osapublishing.org/oe/abstract.cfm?uri=oe-21-23-28862`. Publisher: Optical Society of America.

[6] Yi, X., Yang, Q.-F., Yang, K. Y. & Vahala, K. Theory and measurement of the soliton self-frequency shift and efficiency in optical microcavities. *Optics Letters* **41**, 3419–3422 (2016). URL `https://www.osapublishing.org/ol/abstract.cfm?uri=ol-41-15-3419`. Publisher: Optical Society of America.

[7] Hasegawa, A. Soliton-based optical communications: an overview. *IEEE Journal of Selected Topics in Quantum Electronics* **6**, 1161–1172 (2000). Conference Name: IEEE Journal of Selected Topics in Quantum Electronics.

[8] Leo, F. *et al.* Temporal cavity solitons in one-dimensional Kerr media as bits in an all-optical buffer. *Nature Photonics* **4**, 471–476 (2010). URL `https://www.nature.com/articles/nphoton.2010.120`.

[9] Coen, S. & Erkintalo, M. Universal scaling laws of Kerr frequency combs. *Optics Letters* **38**, 1790–1792 (2013). URL `https://www.osapublishing.org/ol/abstract.cfm?uri=ol-38-11-1790`. Publisher: Optical Society of America.

[10] Del'Haye, P., Beha, K., Papp, S. B. & Diddams, S. A. Self-Injection Locking and Phase-Locked States in Microresonator-Based Optical Frequency Combs. *Physical Review Letters* **112**, 043905 (2014). URL `https://link.aps.org/doi/10.1103/PhysRevLett.112.043905`. Publisher: American Physical Society.

[11] Jang, J. K. *et al.* Synchronization of coupled optical microresonators. *Nature Photonics* **12**, 688–693 (2018). URL `https://www.nature.com/articles/s41566-018-0261-x`.

[12] Erkintalo, M., Murdoch, S. G. & Coen, S. Phase and intensity control of dissipative Kerr cavity solitons. *Journal of the Royal Society of New Zealand* **0**, 1–19 (2021). URL `https://doi.org/10.1080/03036758.2021.1900296`. Publisher: Taylor & Francis _eprint: https://doi.org/10.1080/03036758.2021.1900296.

[13] Li, Z., Xu, Y., Coen, S., Murdoch, S. G. & Erkintalo, M. Experimental observations of bright dissipative cavity solitons

and their collapsed snaking in a Kerr resonator with normal dispersion driving. *Optica* **7**, 1195 (2020). URL https://www.osapublishing.org/abstract.cfm?URI=optica-7-9-1195.
